# Supplementary material for: Unsupervised Pose Flow Learning for Pose Guided Synthesis
Source: arXiv:1909.13819 source file (2019-09-30)
Supplement: Supplementary file 1 [file appendices.tex]

\appendices
\section{Proof of the First Zonklar Equation}
Appendix one text goes here.

% you can choose not to have a title for an appendix
% if you want by leaving the argument blank
\section{}
Appendix two text goes here.
